# Supplementary material for: MixTTA: Low-Rank Cross-Channel Mixing for Reliable Test-Time Adaptation
Source: arXiv:2606.28142 source file (2026-06-30)
Supplement: Supplementary file 1 [file supple.tex]

\documentclass[runningheads]{llncs}

% ---------------------------------------------------------------
% Include basic ECCV package
 
% TODO REVIEW: Insert your submission number below by replacing '*****'
% TODO FINAL: Comment out the following line for the camera-ready version
%\usepackage[review,year=2026,ID=6689]{eccv}
% TODO FINAL: Un-comment the following line for the camera-ready version
\usepackage{eccv}

% OPTIONAL: Un-comment the following line for a version which is easier to read
% on small portrait-orientation screens (e.g., mobile phones, or beside other windows)
%\usepackage[mobile]{eccv}

% ---------------------------------------------------------------
% Other packages

% Commonly used abbreviations (\eg, \ie, \etc, \cf, \etal, etc.)
\usepackage{eccvabbrv}

% Include other packages here, before hyperref.
\usepackage{graphicx}
\usepackage{booktabs}
\usepackage{subcaption}
\usepackage{wrapfig}
\captionsetup[table]{skip=6pt} 
% The "axessiblity" package can be found at: https://ctan.org/pkg/axessibility?lang=en
%\usepackage[accsupp]{axessibility}  % Improves PDF readability for those with disabilities.

\input{preamble}
% ---------------------------------------------------------------
% Hyperref package

% It is strongly recommended to use hyperref, especially for the review version.
% Please disable hyperref *only* if you encounter grave issues.
% hyperref with option pagebackref eases the reviewers' job, but should be disabled for the final version.
%
% If you comment hyperref and then uncomment it, you should delete
% main.aux before re-running LaTeX.
% (Or just hit 'q' on the first LaTeX run, let it finish, and you
%  should be clear).

% TODO FINAL: Comment out the following line for the camera-ready version
%\usepackage[pagebackref,breaklinks,colorlinks,citecolor=eccvblue]{hyperref}
% TODO FINAL: Un-comment the following line for the camera-ready version
\usepackage{hyperref}

% Support for ORCID icon
\usepackage{orcidlink}

\newcommand\samethanks[1][\value{footnote}]{\footnotemark[#1]}

\begin{document}

% ---------------------------------------------------------------
% TODO REVIEW: Replace with your title
\title{Supplementary Material for MixTTA: Low-Rank Cross-Channel Mixing for Reliable Test-Time Adaptation} 

% TODO REVIEW: If the paper title is too long for the running head, you can set
% an abbreviated paper title here. If not, comment out.
\titlerunning{Supplementary Material for MixTTA}

% TODO FINAL: Replace with your author list. 
% Include the authors' OCRID for the camera-ready version, if at all possible.
\author{Mansoo Jung\inst{1}\orcidlink{0009-0003-7846-6521} \and
Youngwook Kim\inst{2}\thanks{Corresponding authors.}\orcidlink{0009-0005-5722-7286} \and
Jungwoo Lee\inst{1, 3}\samethanks\orcidlink{0000-0002-6804-980X}}

% TODO FINAL: Replace with an abbreviated list of authors.
\authorrunning{M. Jung et al.}
% First names are abbreviated in the running head.
% If there are more than two authors, 'et al.' is used.

% TODO FINAL: Replace with your institution list.
\institute{
Seoul National University, Seoul, Republic of Korea \\ 
\email{\{tlwh1179, junglee\}@snu.ac.kr}
\and
Kookmin University, Seoul, Republic of Korea \\
\email{youngwook@kookmin.ac.kr}
\and
HodooAI Labs, Seoul, Republic of Korea \\
}
\maketitle

\section{Experiments on ResNet Backbone}

\subsection{Implementation Details for ResNet Experiments}
In addition to the main ViT results, we also evaluated MixTTA using a ResNet backbone. 
We adopted ResNet models with Group Normalization~\cite{wu2018group}, using pretrained weights from the \texttt{timm} library~\cite{rw2019timm}. 
The learning rate was set to 0.00025; it was doubled in the batch size~1 setting to compensate for the lack of reliable batch statistics, and halved for the affine parameters $(\gamma, \beta)$ in the mixed-shift setting. 
MixTTA modules were inserted into the normalization layers in the stem and the first two residual stages, excluding shortcut connections. 
Unless otherwise specified, we followed the experimental protocol used in the main paper.

\subsection{Results on ImageNet-C}
\begin{table*}[t]
\centering
\small
\setlength{\tabcolsep}{1mm}
\resizebox{\textwidth}{!}{%
\begin{tabular}{l|ccc|cccc|cccc|cccc|c}
\multirow{2}{*}{\textbf{Mild}} & \multicolumn{3}{c|}{\textbf{Noise}} & \multicolumn{4}{c|}{\textbf{Blur}} & \multicolumn{4}{c|}{\textbf{Weather}} & \multicolumn{4}{c|}{\textbf{Digital}} & \multirow{2}{*}{\textbf{Avg.}} \\
\cline{2-16}
& Gauss. & Shot & Impulse & Defocus & Glass & Motion & Zoom & Snow & Frost & Fog & Brit. & Contr. & Elastic & Pixel & JPEG & \\
\hline
No Adapt. & 22.1 & 23.0 & 22.0 & 19.8 & 11.4 & 21.5 & 25.0 & 40.3 & 47.0 & 34.0 & 68.8 & 36.2 & 18.5 & 29.2 & 52.6 & 31.4 \\
\hline
$\bullet$ LinearTCA    & 23.6 & 24.5 & 23.5 & 20.8 & 12.6 & 23.6 & 26.6 & 43.1 & 48.0 & 38.7 & 69.5 & 39.0 & 21.4 & 30.2 & 53.7 & 33.3$\pm${0.0} \\
\hline
$\bullet$ LinearTCA$^+$    & 42.7 & 44.5 & 43.8 & \textbf{25.6} & 26.1 & 41.3 & \textbf{42.5} & 52.1 & 50.5 & 58.8 & 73.3 & 51.4 & 45.3 & 58.4 & \textbf{59.4} & 47.7$\pm${0.1} \\
\hline
$\bullet$ Tent         & 23.1 & 28.2 & 24.8 & 14.9 & 6.8  & 21.8 & 22.6 & \textbf{26.8} & 33.1 & 3.5  & 69.9 & 42.2 & 11.5 & 48.4 & 54.5 & 28.8$\pm${0.2} \\
\rowcolor{lightgray}
~~~+MixTTA  & \textbf{30.8} & \textbf{34.3} & \textbf{31.8} & \textbf{16.7} & \textbf{14.4} & \textbf{26.8} & \textbf{30.3} & 26.4 & \textbf{36.4} & \textbf{4.0}  & \textbf{70.9} & \textbf{44.3} & \textbf{11.8} & \textbf{51.3} & \textbf{55.8} & \textbf{32.4}$\pm${0.5} \\

\hline
$\bullet$ EATA         & 38.9 & 40.9 & 40.0 & \textbf{28.2} & 26.7 & 36.7 & 39.0 & 50.8 & \textbf{49.0} & 55.1 & 71.8 & \textbf{50.0} & 41.7 & \textbf{55.9} & \textbf{58.2} & 45.5$\pm${0.1} \\
\rowcolor{lightgray}
~~~+MixTTA  & \textbf{40.4} & \textbf{42.8} & \textbf{41.7} & 27.4 & \textbf{27.5} & \textbf{39.2} & \textbf{41.4} & \textbf{51.1} & 47.9 & \textbf{55.5} & \textbf{72.3} & 49.0 & \textbf{44.8} & 55.4 & 57.1 & \textbf{46.2}$\pm${0.3} \\
\hline
$\bullet$ SAR          & 32.1 & 34.1 & 33.3 & 18.5 & 18.6 & 30.4 & 30.5 & \textbf{42.5} & 43.4 & \textbf{40.9} & 70.3 & 44.0 & \textbf{15.5} & 49.0 & 55.3 & 37.2$\pm${0.7} \\
\rowcolor{lightgray}
~~~+MixTTA   & \textbf{33.7} & \textbf{36.0} & \textbf{34.9} & \textbf{18.8} & \textbf{20.3} & \textbf{31.5} & \textbf{31.9} & 41.8 & \textbf{43.6} & 34.6 & \textbf{70.5} & \textbf{44.4} & 13.9 & \textbf{50.5} & \textbf{55.5} & \textbf{37.5}$\pm${1.6} \\
\hline
$\bullet$ DeYO         & 41.0 & 43.1 & 42.2 & 22.8 & 24.5 & 38.9 & 27.8 & 51.5 & 49.9 & \textbf{56.3} & 73.0 & 50.5 & 43.1 & 56.5 & \textbf{58.1} & \textbf{45.3}$\pm${0.5} \\
\hline
\rowcolor{lightgray}
~~~+MixTTA  & \textbf{42.9} & \textbf{44.9} & \textbf{44.1} & \textbf{23.7} & \textbf{25.2} & \textbf{40.4} & \textbf{36.3} & \textbf{52.4} & \textbf{50.5} & 20.2 & \textbf{73.2} & \textbf{51.1} & \textbf{46.0} & \textbf{57.8} & 58.0 & 44.4$\pm${2.2} \\
\hline
$\bullet$ ReCAP        & 41.8 & 43.6 & 43.0 & 24.3 & 25.4 & 40.3 & \textbf{40.7} & 51.9 & 50.2 & 57.1 & 73.1 & 51.0 & 43.5 & 57.1 & 58.4 &  46.8$\pm${0.1} \\
\rowcolor{lightgray}
~~~+MixTTA & \textbf{43.4} & \textbf{45.3} & \textbf{44.4} & \textbf{25.2} & \textbf{26.6} & \textbf{41.7} & 40.4 & \textbf{52.9} & \textbf{51.2} & \textbf{59.8} & \textbf{73.4} & \textbf{51.5} & \textbf{46.8} & \textbf{58.4} & 58.4 & \textbf{47.9}$\pm${0.1}

\end{tabular}
}
\caption{
Comparisons with baselines on ImageNet-C at severity level 5 under the mild scenario regarding accuracy (\%). \textbf{Bold} values denote the top-performing results.}
\label{tab:comparison mild}
\end{table*}

\subsubsection{Comparison on Mild Scenario}

Table~\ref{tab:comparison mild} summarizes the results on ImageNet-C at severity level~5 under the mild scenario. Overall, MixTTA serves as an effective plug-in module for most baseline TTA methods. In particular, it improves the average accuracy of most baselines, yielding gains of +3.6\%p for Tent, +0.7\%p for EATA, +0.3\%p for SAR, and +1.1\%p for ReCAP. Although the average accuracy of DeYO decreases, MixTTA still improves DeYO on 13 out of 15 corruption types, with only \textit{Fog} and \textit{JPEG} showing performance drops. The gains are most consistent on \textit{Noise} corruptions, where MixTTA substantially strengthens all baselines. For example, for Tent, MixTTA improves the accuracy from 23.1\% to 30.8\% on \textit{Gaussian}, from 28.2\% to 34.3\% on \textit{Shot}, and from 24.8\% to 31.8\% on \textit{Impulse}. A similar trend is observed for ReCAP, where MixTTA improves all three noise types and further boosts several \textit{Weather} and \textit{Digital} corruptions, such as \textit{Pixel} (57.1\% $\rightarrow$ 58.4\%). Notably, MixTTA improves the average accuracy from 46.8\% to 47.9\%, exceeding the gain obtained by applying LinearTCA to the same base method (\ie, LinearTCA$^+$, 47.7\%). These results suggest that MixTTA is particularly effective when the baseline remains vulnerable to corruption-induced cross-channel perturbations.

\begin{table*}[t]
\centering
\small
\setlength{\tabcolsep}{1mm}
\resizebox{\textwidth}{!}{%
\begin{tabular}{l|ccc|cccc|cccc|cccc|c}
\multirow{2}{*}{\textbf{Label Shifts}} & \multicolumn{3}{c|}{\textbf{Noise}} & \multicolumn{4}{c|}{\textbf{Blur}} & \multicolumn{4}{c|}{\textbf{Weather}} & \multicolumn{4}{c|}{\textbf{Digital}} & \multirow{2}{*}{\textbf{Avg.}} \\
\cline{2-16}
& Gauss. & Shot & Impulse & Defocus & Glass & Motion & Zoom & Snow & Frost & Fog & Brit. & Contr. & Elastic & Pixel & JPEG & \\
\hline
No Adapt.          & 22.1 & 23.0 & 22.0 & 19.8 & 11.4 & 21.5 & 25.0 & 40.3 & 47.0 & 34.0 & 68.8 & 36.2 & 18.5 & 29.2 & 52.6 & 31.4  \\
\hline
$\bullet$ LinearTCA    & 23.9 & 24.9 & 23.8 & 21.0 & 12.7 & 23.7 & 26.9 & 43.5 & 48.5 & \textbf{38.1} & 69.4 & 39.4 & 21.9 & 30.4 & 54.0 & 33.5$\pm${0.0} \\
\hline
$\bullet$ LinearTCA$^+$    & \textbf{44.1} & 46.0 & \textbf{44.9} & \textbf{27.1} & 10.5 & \textbf{43.7} & \textbf{37.9} & 54.1 & \textbf{52.9} & 25.8 & \textbf{73.5} & \textbf{54.1} & \textbf{42.8} & 61.4 & \textbf{60.7} & \textbf{45.3}$\pm${3.8} \\
\hline
$\bullet$ Tent         & 13.8 & 19.7 & 15.6 & 13.3 & 7.6  & 17.3 & 18.6 & \textbf{17.3} & \textbf{21.3} & 2.1  & 69.9 & 42.0 & \textbf{6.2}  & 49.3 & 53.9 & 24.5$\pm${0.6} \\
\rowcolor{lightgray}
~~~+MixTTA   & \textbf{22.1} & \textbf{38.2} & \textbf{31.0} & \textbf{16.7} & \textbf{14.1} & \textbf{27.2} & \textbf{31.2} & 13.7 & 19.4 & \textbf{2.7}  & \textbf{72.1} & \textbf{46.6} & 5.7  & \textbf{53.6} & \textbf{56.6} & \textbf{30.0}$\pm${1.1} \\
\hline
$\bullet$ EATA         & 29.2 & 31.6 & 30.4 & 18.0 & 17.3 & 28.5 & 29.2 & 44.4 & \textbf{44.2} & 41.6 & 70.6 & \textbf{44.1} & 26.8 & 46.8 & \textbf{55.7} & 33.1$\pm${0.6} \\
\rowcolor{lightgray}
~~~+MixTTA   & \textbf{35.3} & \textbf{39.2} & \textbf{37.0} & \textbf{20.0} & \textbf{21.6} & \textbf{33.2} & \textbf{35.4} & 44.4 & 42.1 & \textbf{52.1} & \textbf{70.8} & 43.7 & \textbf{37.6} & \textbf{52.0} & 54.4 & \textbf{41.3}$\pm${0.2} \\
\hline
$\bullet$ SAR          & 36.1 & 38.5 & 37.7 & 18.5 & 15.0 & 33.6 & 27.9 & \textbf{25.1} & 45.0 & 31.5 & 71.4 & 47.0 & \textbf{6.3}  & 52.4 & 56.5 & 36.2$\pm${1.7} \\
\rowcolor{lightgray}
~~~+MixTTA   & \textbf{37.9} & \textbf{40.1} & \textbf{38.7} & 18.5 & \textbf{20.8} & \textbf{34.5} & \textbf{35.4} & 21.5 & \textbf{45.3} & \textbf{35.3} & \textbf{71.7} & \textbf{47.4} & 5.8  & \textbf{53.5} & 56.5 & \textbf{37.5}$\pm${2.0} \\
\hline
$\bullet$ DeYO         & 42.7 & 45.0 & 43.7 & \textbf{21.8} & \textbf{16.3} & 41.1 & \textbf{14.3} & 52.6 & 50.8 & 20.3 & 73.2 & 52.4 & 42.3 & 59.6 & \textbf{59.2} & \textbf{42.3}$\pm${0.1} \\
\rowcolor{lightgray}
~~~+MixTTA   & \textbf{43.6} & \textbf{45.9} & \textbf{44.8} & 18.5 & 8.7  & \textbf{42.9} & 7.7  & \textbf{53.3} & \textbf{51.0} & \textbf{20.4} & \textbf{73.3} & \textbf{52.9} & \textbf{49.2} & \textbf{60.5} & 59.1 & 42.1$\pm${3.3} \\
\hline
$\bullet$ ReCAP        & 42.9 & 45.0 & 43.9 & 23.9 & 8.9 & 42.8 & \textbf{24.0} & 53.4 & \textbf{52.1} & 20.3 & 73.4 & 53.2 & 29.8 & 60.6 & 59.9 & 42.3$\pm$1.9 \\
\rowcolor{lightgray}
~~~+MixTTA   & \textbf{43.7} & \textbf{46.2} & \textbf{44.5} & \textbf{24.4} & \textbf{16.8} & \textbf{43.7} & 18.8 & \textbf{54.2} & 51.9 & \textbf{20.7} & 73.4 & \textbf{53.6} & \textbf{39.9} & \textbf{61.7} & 59.9 & \textbf{43.6}$\pm$2.8\\

\hline

\end{tabular}
}
\caption{
Comparisons with baselines on ImageNet-C at severity level 5 under online imbalanced label shifts with imbalance ratio $\infty$ regarding accuracy (\%).}
\label{tab:comparison label shifts}
\end{table*}

\begin{table*}[t]
\centering
\small
\setlength{\tabcolsep}{1mm}
\resizebox{\textwidth}{!}{%
\begin{tabular}{l|ccc|cccc|cccc|cccc|c}
\multirow{2}{*}{\textbf{Batch Size 1}} & \multicolumn{3}{c|}{\textbf{Noise}} & \multicolumn{4}{c|}{\textbf{Blur}} & \multicolumn{4}{c|}{\textbf{Weather}} & \multicolumn{4}{c|}{\textbf{Digital}} & \multirow{2}{*}{\textbf{Avg.}} \\
\cline{2-16}
& Gauss. & Shot & Impulse & Defocus & Glass & Motion & Zoom & Snow & Frost & Fog & Brit. & Contr. & Elastic & Pixel & JPEG & \\
\hline
No Adapt.          & 22.1 & 23.0 & 22.0 & 19.8 & 11.4 & 21.5 & 25.0 & 40.3 & 47.0 & 34.0 & 68.8 & 36.2 & 18.5 & 29.2 & 52.6 & 31.4  \\
\hline
$\bullet$ LinearTCA    & 23.6 & 24.5 & 23.5 & 20.8 & 12.6 & 23.6 & 26.6 & 43.1 & 48.1 & \textbf{38.7} & 69.5 & 39.0 & 21.5 & 30.2 & 53.8 & 33.3$\pm$0.0 \\
\hline
$\bullet$ LinearTCA$^+$    & 44.0 & 46.2 & 45.1 & \textbf{28.5} & 27.8 & 44.2 & \textbf{42.9} & 56.6 & 53.6 & 22.3 & 73.6 & 55.2 & 43.0 & 62.4 & \textbf{61.3} & 47.1$\pm$0.4 \\
\hline
$\bullet$ Tent         & 11.3 & 20.7 & 14.6 & 13.1 & 3.5 & 18.6 & 18.5 & \textbf{15.6} & \textbf{20.1} & \textbf{1.5} & 69.8 & 42.1 & \textbf{6.5} & 49.4 & 53.8 & 23.9$\pm$0.3 \\
\rowcolor{lightgray}
~~~+MixTTA   & \textbf{25.4} & \textbf{39.0} & \textbf{35.6} & \textbf{16.0} & \textbf{10.6} & \textbf{28.9} & \textbf{28.7} & 13.3 & 19.9 & 1.4  & \textbf{72.2} & \textbf{46.5} & 5.9  & \textbf{53.7} & \textbf{56.5} & \textbf{30.2}$\pm$0.7 \\
\hline
$\bullet$ EATA         & 29.2 & 31.6 & 30.4 & 18.0 & 17.3 & 28.5 & 29.2 & 44.4 & 44.2 & 41.6 & 70.6 & 44.1 & 26.8 & 46.8 & 55.7 & 37.2$\pm$0.1 \\
\rowcolor{lightgray}
~~~+MixTTA   & \textbf{34.6} & \textbf{37.9} & \textbf{35.9} & \textbf{19.3} & \textbf{20.5} & \textbf{33.7} & \textbf{35.1} & \textbf{48.8} & \textbf{45.4} & \textbf{46.7} & \textbf{72.2} & \textbf{46.6} & \textbf{37.0} & \textbf{52.7} & \textbf{56.4} & \textbf{41.5}$\pm$0.3 \\
\hline
$\bullet$ SAR          & 28.7 & 30.9 & 29.2 & 18.4 & 15.1 & 28.7 & 30.5 & 44.9 & 44.4 & 33.7 & 72.0 & 44.7 & \textbf{14.6} & 47.6 & 56.3 & 36.0$\pm$0.0 \\
\rowcolor{lightgray}
~~~+MixTTA   & \textbf{29.9} & \textbf{32.6} & \textbf{30.6} & \textbf{18.5} & \textbf{17.0} & \textbf{29.9} & \textbf{31.5} & \textbf{45.4} & \textbf{44.6} & \textbf{33.9} & \textbf{72.2} & \textbf{44.8} & 13.5 & \textbf{49.3} & 56.3 & \textbf{36.7}$\pm$0.3 \\
\hline
$\bullet$ DeYO         & 42.9 & 45.2 & 43.9 & 22.8 & 24.0 & 41.8 & 25.5 & 53.9 & 52.1 & \textbf{58.1} & 73.4 & 53.4 & 47.7 & 60.1 & 59.8 & \textbf{47.0}$\pm$0.9 \\
\rowcolor{lightgray}
~~~+MixTTA   & \textbf{44.4} & \textbf{46.5} & \textbf{45.8} & \textbf{22.9} & \textbf{24.9} & \textbf{43.4} & \textbf{32.1} & \textbf{55.1} & \textbf{52.5} & 21.0  & 73.4 & \textbf{54.0} & \textbf{51.2} & \textbf{61.6} & \textbf{59.9} & 45.4$\pm$2.2 \\
\hline
$\bullet$ ReCAP        & 43.3 & 45.7 & 44.5 & 26.4 & 26.8 & 43.5 & \textbf{40.5} & 56.0 & 53.1 & 21.3 & 73.5 & 54.7 & 40.5 & 61.7 & 60.7 & 46.1$\pm$1.5 \\
\rowcolor{lightgray}
~~~+MixTTA   & \textbf{44.5} & \textbf{46.6} & \textbf{45.4} & 26.4 & \textbf{28.5} & \textbf{45.9} & 32.9 & \textbf{57.0} & \textbf{53.7} & \textbf{21.7} & \textbf{73.6} & \textbf{55.3} & \textbf{53.9} & \textbf{63.1} & \textbf{60.9} & \textbf{47.3}$\pm$2.7 \\

\hline
\end{tabular}
}
\caption{
Comparisons with baselines on ImageNet-C at severity level 5 under batch size 1 regarding accuracy (\%).
}
\label{tab:comparison batch size 1}
\end{table*}

\subsubsection{Comparison on Wild Scenario}

Table~\ref{tab:comparison label shifts} shows that MixTTA remains effective under severe online imbalanced label shifts. It improves four of the five baselines in terms of average accuracy, with especially large gains for Tent (+5.5\%p) and EATA (+8.2\%p). ReCAP+MixTTA achieves the best average accuracy of 43.6\%. Although several corruption types still exhibit performance drops, such cases are limited and mostly occur in regimes where the original baseline adaptation is already unstable. This suggests that the observed degradations are more likely attributable to baseline fragility under skewed target streams than to MixTTA itself.

Table~\ref{tab:comparison batch size 1} reports the results on ImageNet-C at severity level~5 under batch size~1, where adaptation must rely solely on instance-level statistics. Even in this highly constrained setting, MixTTA improves the average accuracy of all baselines except DeYO. The gains are particularly notable for Tent and EATA, whose average accuracies increase from 23.9\% to 30.2\% and from 37.2\% to 41.5\%, respectively. Moreover, ReCAP+MixTTA achieves the best overall average accuracy of 47.3\%, slightly outperforming LinearTCA$^+$ (47.1\%). The improvements are broadly distributed across corruption types, particularly across several \textit{Noise}, \textit{Blur}, and \textit{Digital} corruptions, indicating that MixTTA remains effective even when reliable batch statistics are unavailable.

Table~\ref{tab:comparison_mix} summarizes the results under the mixed-shift setting, where multiple corruption types are combined within a single batch. In this setting, MixTTA improves four out of five baselines, yielding gains of +2.4\%p for EATA, +0.8\%p for SAR, +2.9\%p for DeYO, and +1.1\%p for ReCAP, with Tent being the only exception. These results suggest that MixTTA remains effective even when the target batch contains heterogeneous corruption patterns, where adaptation must cope with more entangled feature shifts. Compared with LinearTCA$^+$, whose gain is marginal in this setting, MixTTA appears more robust under mixed shifts, likely because its feature correction is driven by the current test-time feature statistics rather than by a fixed correlation-alignment target.

\begin{table}[!t]
\centering

\begin{minipage}[t]{0.48\linewidth}
\centering
\small
\scalebox{0.84}{%
\begin{tabular}{l|c}
\rowcolor{white}
\textbf{Mixed Shifts} & \textbf{Accuracy (\%)} \\
\hline
No adapt. & 31.4 \\
\hline
$\bullet$ LinearTCA & 33.9$\pm$0.0 \\
\hline
$\bullet$ LinearTCA$^+$ & 43.0$\pm$0.2 \\
\hline
$\bullet$ Tent & \textbf{14.1}$\pm$0.5 \\
\rowcolor{lightgray}
~~~+ MixTTA  & 10.5$\pm$4.6 \\
\hline
$\bullet$ EATA & 38.3$\pm$0.2 \\
\rowcolor{lightgray}
~~~+ MixTTA  & \textbf{40.7}$\pm$0.1 \\
\hline
$\bullet$ SAR & 37.5$\pm$0.1 \\
\rowcolor{lightgray}
~~~+ MixTTA  & \textbf{38.3}$\pm$0.0 \\
\hline
$\bullet$ DeYO & 37.2$\pm$0.5 \\
\rowcolor{lightgray}
~~~+ MixTTA  & \textbf{40.1}$\pm$1.6 \\
\hline
$\bullet$ ReCAP & 42.1$\pm$0.3 \\
\rowcolor{lightgray}
~~~+ MixTTA  & \textbf{43.2}$\pm$0.2 \\
\end{tabular}
}
\caption{Comparisons with baselines on ImageNet-C at severity level 5 under a mixture of 15 types of corruption regarding accuracy (\%).}
\label{tab:comparison_mix}
\end{minipage}
\hfill
\begin{minipage}[t]{0.50\linewidth}
\centering
\small
\setlength{\tabcolsep}{1mm}
\resizebox{\linewidth}{!}{%
\begin{tabular}{l|c|c|c}
\rowcolor{white}
{\makecell{\textbf{ImageNet}\\{\textbf{-Sketch}}}} & \textbf{Mild} & \textbf{Label Shifts} & \textbf{Batch Size 1} \\
\hline
No Adapt. & 29.2 & 29.6 & 29.2 \\
\hline
$\bullet$ LinearTCA & 30.9$\pm$0.0 & 31.7$\pm$0.0 & 30.9$\pm$0.0 \\
\hline
$\bullet$ LinearTCA$^+$ & \textbf{37.9}$\pm$0.2 & 38.1$\pm$0.5 & 38.3$\pm$0.3 \\ 
\hline
$\bullet$ Tent & 30.8$\pm$0.1 & 32.3$\pm$0.4 & 28.5$\pm$5.6 \\
\rowcolor{lightgray}
~~~+ MixTTA & \textbf{31.1}$\pm$0.2 & \textbf{32.7}$\pm$0.8 & \textbf{32.0}$\pm$0.2 \\
\hline
$\bullet$ EATA & 34.7$\pm$0.1 & 32.7$\pm$0.6 & 29.5$\pm$0.0 \\
\rowcolor{lightgray}
~~~+ MixTTA & \textbf{35.6}$\pm$0.1 & \textbf{33.3}$\pm$0.2 & \textbf{33.3}$\pm$0.1 \\
\hline
$\bullet$ SAR & 30.2$\pm$0.1 & 31.7$\pm$0.4 & 31.1$\pm$0.4 \\
\rowcolor{lightgray}
~~~+ MixTTA & \textbf{31.6}$\pm$0.3 & \textbf{33.4}$\pm$0.1 & \textbf{33.8}$\pm$0.5 \\
\hline
$\bullet$ DeYO & 35.5$\pm$0.4 & 36.9$\pm$0.6 & 37.3$\pm$0.8 \\
\rowcolor{lightgray}
~~~+ MixTTA & \textbf{36.0}$\pm$0.7 & \textbf{37.2}$\pm$0.4 & \textbf{37.7}$\pm$0.4 \\
\hline
$\bullet$ ReCAP & 36.3$\pm$0.3 & 38.0$\pm$0.5 & 38.0$\pm$0.3 \\
\rowcolor{lightgray}
~~~+ MixTTA & \textbf{36.8}$\pm$0.6 & \textbf{38.3}$\pm$0.2 & \textbf{38.6}$\pm$0.1 \\
\end{tabular}
}
\caption{Comparisons with baselines on ImageNet-Sketch under mild and wild scenarios regarding accuracy (\%).}
\label{tab:comparison_imagenet_sketch}
\end{minipage}

\end{table}

\subsubsection{Results on ImageNet-Sketch}

Table~\ref{tab:comparison_imagenet_sketch} reports the accuracy on ImageNet-Sketch under the mild setting and two wild settings. Overall, MixTTA consistently improves all five baseline TTA methods across all three scenarios. While the gains are relatively modest in the mild setting, they become more pronounced under the wild regimes, particularly for methods that are more susceptible to challenging online adaptation. For example, under batch size~1, Tent improves from 28.5\% to 32.0\%, while EATA and SAR also show clear gains, increasing from 29.5\% to 33.3\% and from 31.1\% to 33.8\%, respectively. MixTTA also yields consistent improvements for stronger baselines such as DeYO and ReCAP. Moreover, ReCAP+MixTTA surpasses LinearTCA$^+$ under both wild settings, suggesting that MixTTA provides complementary benefits beyond explicit correlation alignment. These results indicate that the cross-channel correction induced by MixTTA is not limited to corruption-based shifts, but also extends effectively to stylized domain gaps such as ImageNet-Sketch.

\section{Sensitivity of $\eta$}

Table~\ref{tab:sensitivity_eta} reports the sensitivity of MixTTA to the projection strength $\eta$ in the spectral projection on ImageNet-C at severity level 5. Overall, the performance remains stable across $\eta \in [0.7, 1.0]$ for all five baselines, indicating that MixTTA is not highly sensitive to the exact choice of this hyperparameter. The best results are generally obtained around $\eta = 0.9$, which yields the highest accuracy for EATA, SAR, and ReCAP, and ties for the best result for DeYO. Tent achieves its best performance at $\eta = 1.0$, although the gap from $\eta = 0.9$ is negligible (55.3\% vs.\ 55.2\%). These results suggest that MixTTA is robust over a broad range of $\eta$ values, while $\eta = 0.9$ serves as a strong default choice across different baseline methods.

\begin{table}[t]
\centering
\small
\setlength{\tabcolsep}{2mm}
\resizebox{0.65\linewidth}{!}{%
\begin{tabular}{r|c|c|c|c}
\multirow{2}{*}{\textbf{Method}} & \multicolumn{4}{c}{$\eta$} \\
\cline{2-5}
 & 0.7 & 0.8 & 0.9 & 1.0 \\
\hline
Tent+MixTTA & 54.1 & 54.3 & 55.2 & \textbf{55.3} \\
EATA+MixTTA & 63.7 & 63.9 & \textbf{64.2} & 64.1 \\
SAR+MixTTA & 56.5 & 57.0 & \textbf{57.4} & 57.1 \\
DeYO+MixTTA & 65.1 & 65.5 & \textbf{65.6} & \textbf{65.6} \\
ReCAP+MixTTA & 64.5 & 64.8 & \textbf{64.9} & 64.8 \\
\end{tabular}%
}
\caption{
Comparison of average accuracy of MixTTA performance with varying $\eta$ values and baselines on ImageNet-C severity level 5.
}
\label{tab:sensitivity_eta}
\end{table}

\section*{Acknowledgements.} 
%This work was supported by Institute of Information \& Communications Technology Planning \& Evaluation(IITP) under AI Star Fellowship(Kookmin University) (RS-2025-02219317) and the Leading Generative AI Human Resources Development (IITP-2026-RS-2026-25546026) grant funded by the Korea government(MSIT), and “Advanced GPU Utilization Support Program” funded by the Government of the Republic of Korea (Ministry of Science and ICT). 
%This work is in part supported by the National Research Foundation of Korea (NRF, RS-2024-00451435(20\%), RS-2024-00413957(20\%)), Institute of Information \& communications Technology Planning \& Evaluation (IITP, RS-2025-02305453(15\%), RS-2025-02273157(15\%), RS-2025-25442149(15\%) RS-2021-II211343(15\%)) grant funded by the Ministry of Science and ICT (MSIT), Institute of New Media and Communications(INMAC), and the BK21 FOUR program of the Education, Artificial Intelligence Graduate School Program (Seoul National University), and Research Program for Future ICT Pioneers, Seoul National University in 2026.
This work was supported by the Institute of Information \&Communications Technology Planning \& Evaluation (IITP) under the AI Star Fellowship (Kookmin University) (RS-2025-02219317 (10\%)) and the Leading Generative AI Human Resources Development (IITP-2026-RS-2026-25546026 (10\%)) grant funded by the Korea government (MSIT), and the ``Advanced GPU Utilization Support Program'' funded by the Government of the Republic of Korea (Ministry of Science and ICT), the National Research Foundation of Korea (NRF, RS-2024-00451435 (10\%), RS-2024-00413957 (10\%)), the Institute of Information \& Communications Technology Planning \& Evaluation (IITP, RS-2025-02305453 (15\%), RS-2025-02273157 (15\%), RS-2025-25442149 (15\%), RS-2021-II211343 (15\%)) grant funded by the Ministry of Science and ICT (MSIT), the Institute of New Media and Communications (INMAC), and the BK21 FOUR program of the Education, the Artificial Intelligence Graduate School Program (Seoul National University), and the Research Program for Future ICT Pioneers, Seoul National University in 2026.

% ---- Bibliography ----
%
% BibTeX users should specify bibliography style 'splncs04'.
% References will then be sorted and formatted in the correct style.
%
\bibliographystyle{splncs04}
\bibliography{supple}
\end{document}
